# Supplementary material for: The role of Si vacancies in the segregation of O, C, and N at silicon grain boundaries: An ab initio study
Source: arXiv:2201.07518 source file (2022-01-19)
Supplement: Supplementary file 1 [file Sigb_CNO_seg_suppmat.pdf]

## Supplementary Material

### The role of Si vacancies in the segregation of O, C and N at silicon grain boundaries: an ab initio study

Rita Maji

*Dipartimento di Scienze e Metodi dell'Ingegneria,*

*Università di Modena e Reggio Emilia,*

*Via Amendola 2 Padiglione Tamburini , I-42122 Reggio Emilia, Italy*

Julia Contreras-García

*Laboratoire de Chimie Théorique, Sorbonne Université and CNRS F-75005 Paris, France*

Nathalie Capron

*Sorbonne Université, CNRS, Laboratoire de Chimie Physique Matière et Rayonnement,*

*UMR 7614, F-75005 Paris, France.*

Elena Degoli\*

*Dipartimento di Scienze e Metodi dell'Ingegneria,*

*Università di Modena e Reggio Emilia,*

*Via Amendola 2 Padiglione Morselli, I-42122 Reggio Emilia, Italy,*

*Centro Interdipartimentale En&Tech,*

*Via Amendola 2 Padiglione Morselli, I-42122 Reggio Emilia, Italy,*

*Centro S3, Istituto Nanoscienze-Consiglio Nazionale delle Ricerche (CNR-NANO),*

*Via Campi 213/A, 41125 Modena, Italy*

Eleonora Luppi<sup>†</sup>

*Laboratoire de Chimie Théorique, Sorbonne Université and CNRS F-75005 Paris, France*

---

\* [elena.degoli@unimore.it](mailto:elena.degoli@unimore.it)

† [eleonora.luppi@sorbonne-universite.fr](mailto:eleonora.luppi@sorbonne-universite.fr)

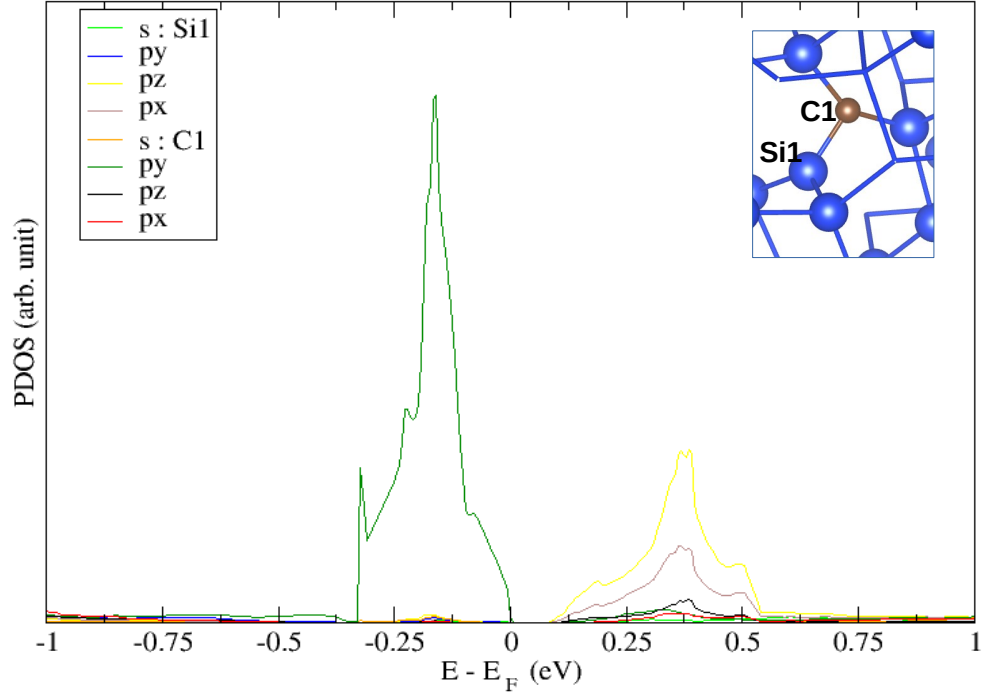

FIG. 1. Projected density of states (PDOS) of the atoms indicated in the inset structure, belonging to the  $\Sigma 3\{111\}$  with one interstitial C atom. The atomic orbitals with larger contributions are plotted here.

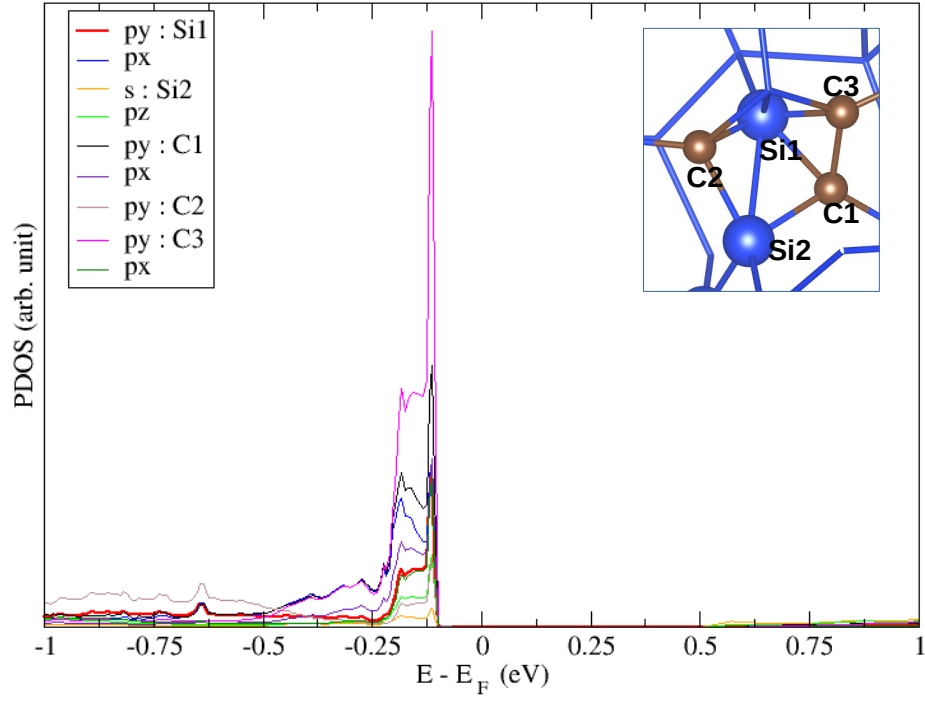

FIG. 2. Density of states (PDOS) of the atoms indicated in the inset structure, belonging to the  $\Sigma 3\{111\}$  with three interstitial C atoms. The atomic orbitals with larger contributions are plotted here.

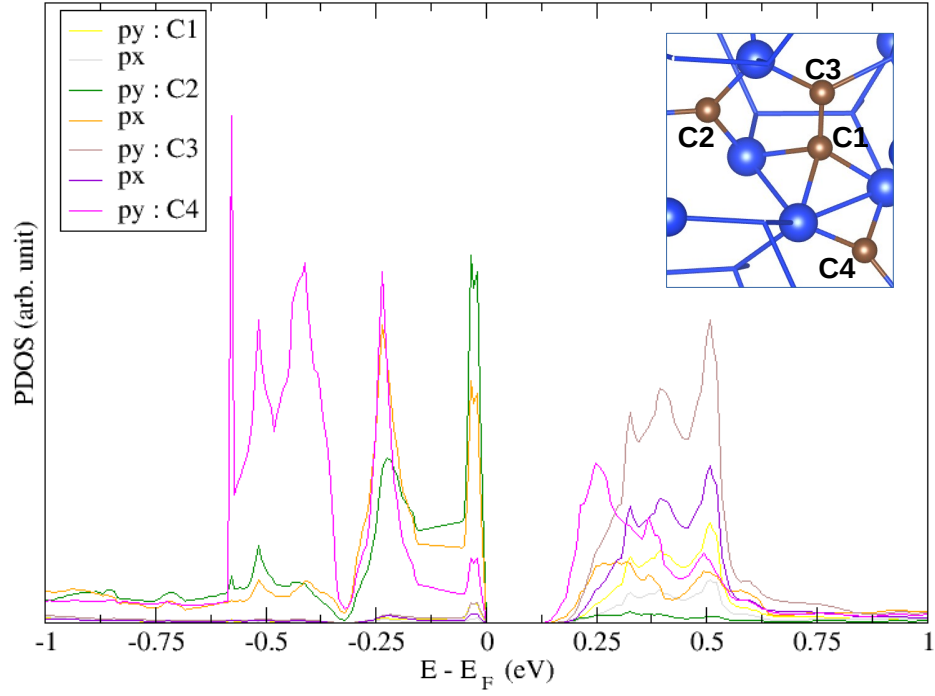

FIG. 3. Projected density of states (PDOS) of the atoms indicated in the inset structure, belonging to the  $\Sigma 3\{111\}$  with four interstitial C atoms. The atomic orbitals with larger contributions are plotted here.

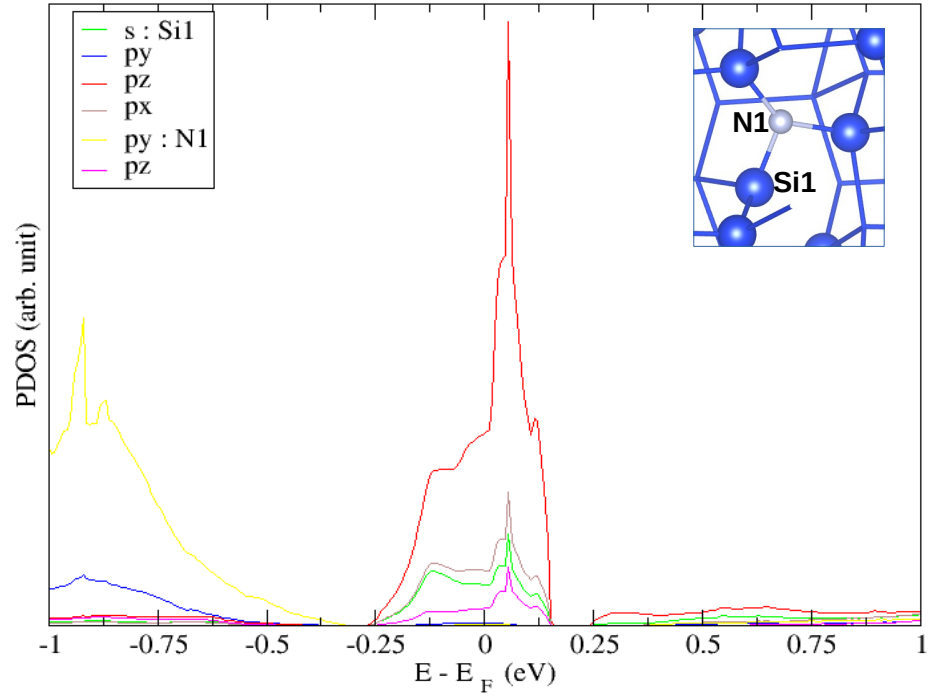

FIG. 4. Projected density of states (PDOS) of the atoms indicated in the inset structure, belonging to the  $\Sigma 3\{111\}$  with one interstitial N atom. The atomic orbitals with larger contributions are plotted here..

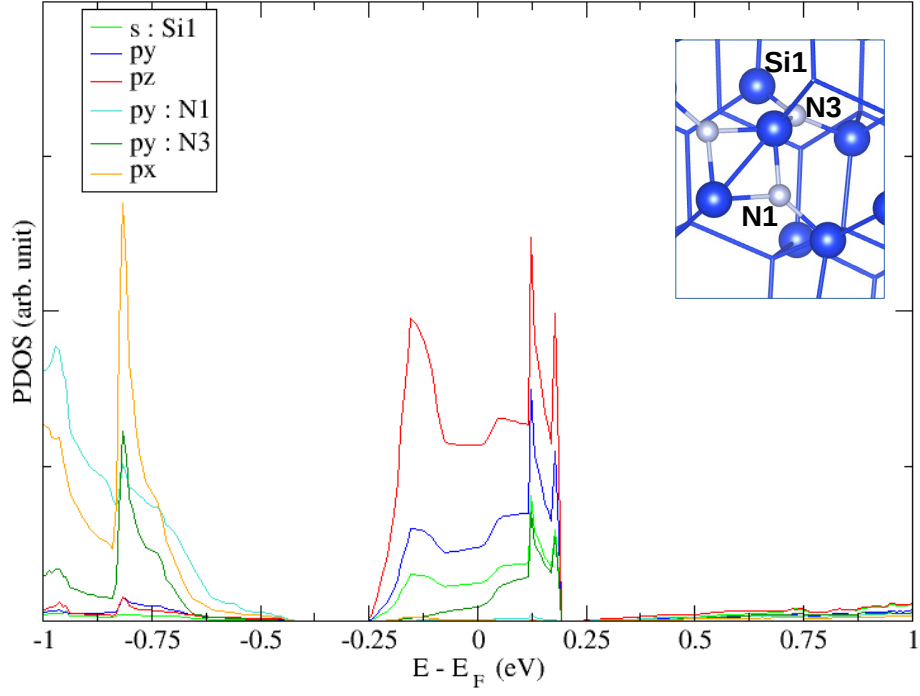

FIG. 5. Projected density of states (PDOS) of the atoms indicated in the inset structure, belonging to the  $\Sigma 3\{111\}$  with three interstitial N atoms. The atomic orbitals with larger contributions are plotted here.

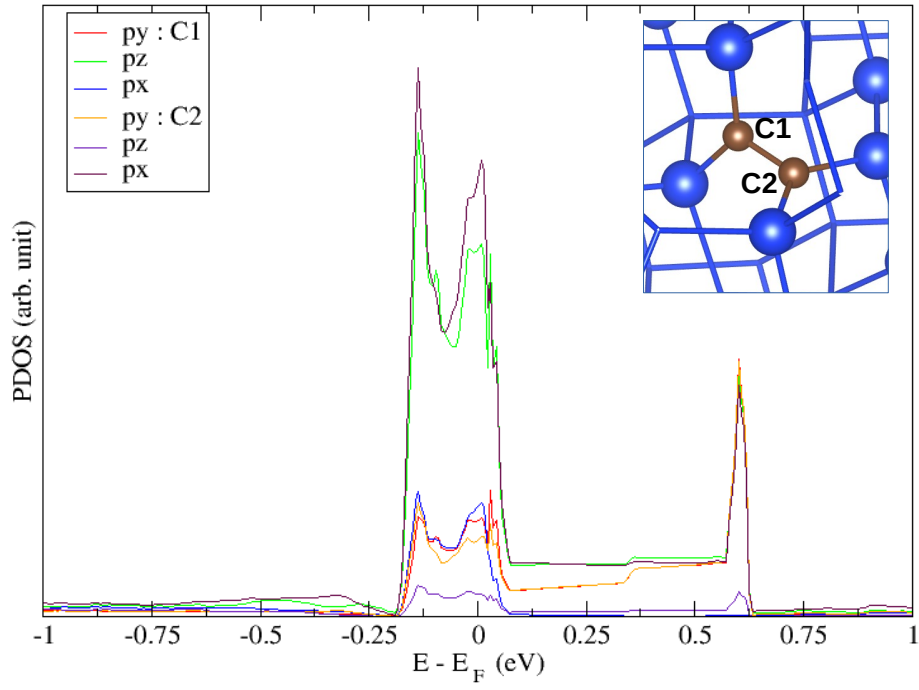

FIG. 6. Projected density of states (PDOS) of the atoms indicated in the inset structure, belonging to the  $\Sigma 3\{111\}$  with two interstitial C atoms in presence of vacancy V1. The atomic orbitals with larger contributions are plotted here.

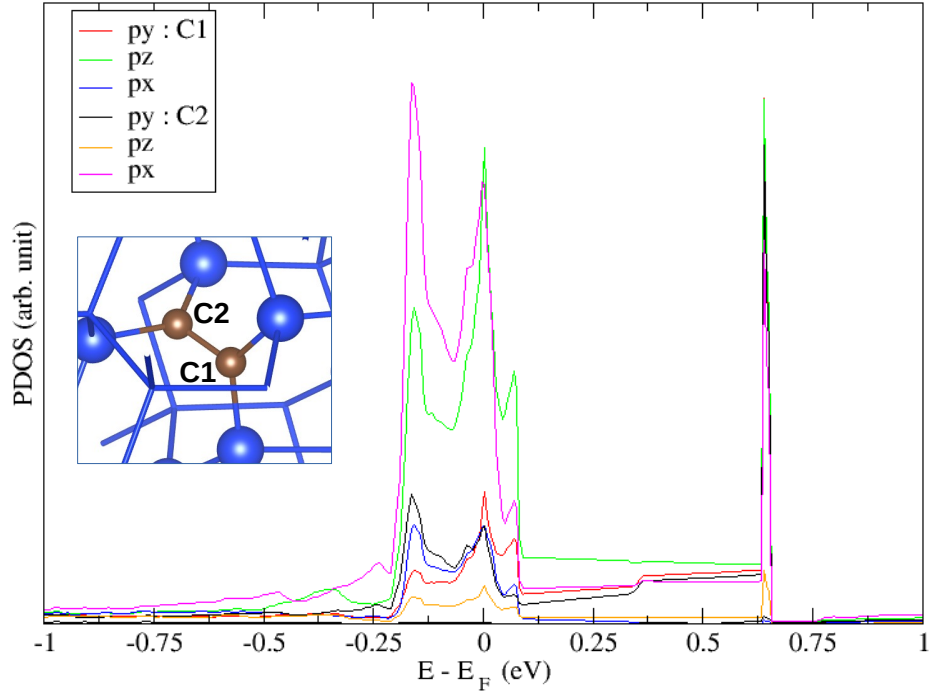

FIG. 7. Projected density of states (PDOS) of the atoms indicated in the inset structure, belonging to the  $\Sigma 3\{111\}$  with two interstitial C atoms in presence of vacancy V2. The atomic orbitals with larger contributions are plotted here.

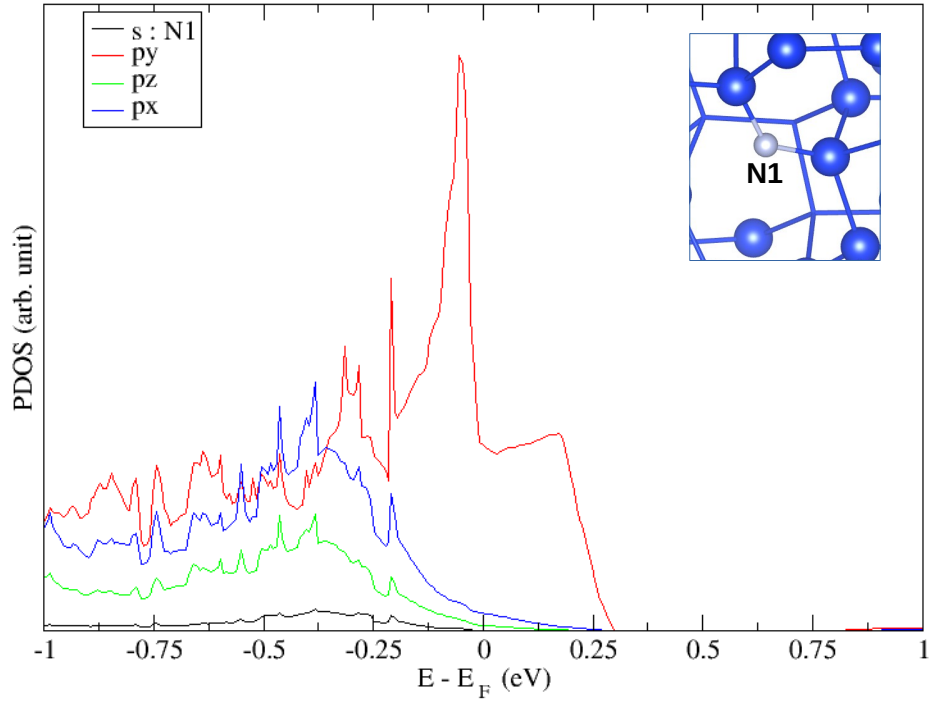

FIG. 8. Projected density of states (PDOS) of the atoms indicated in the inset structure, belonging to the  $\Sigma 3\{111\}$  with one interstitial N atom in presence of vacancy V1. The atomic orbitals with larger contributions are plotted here.

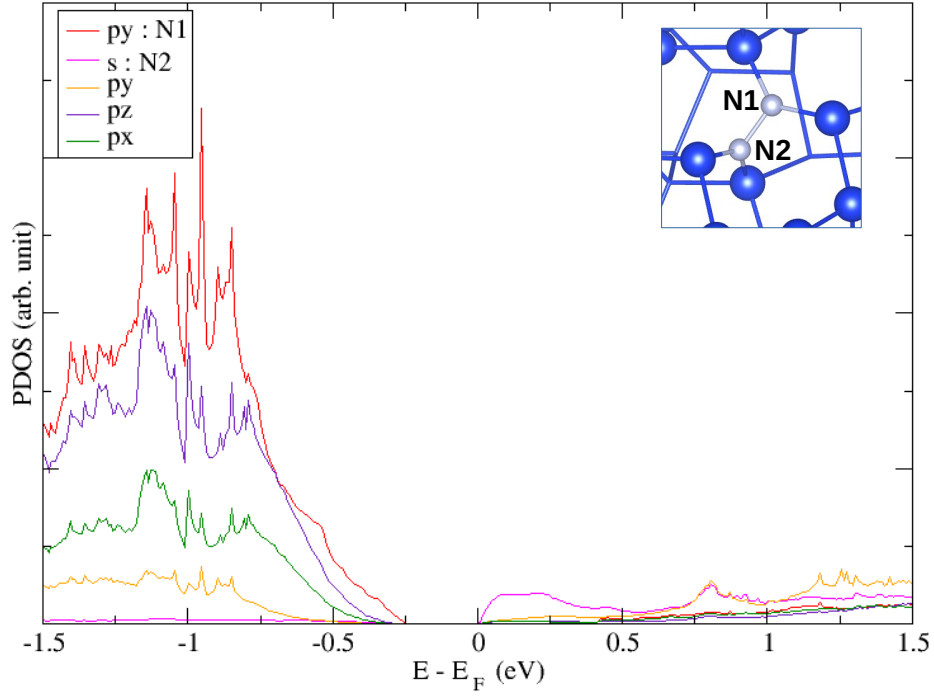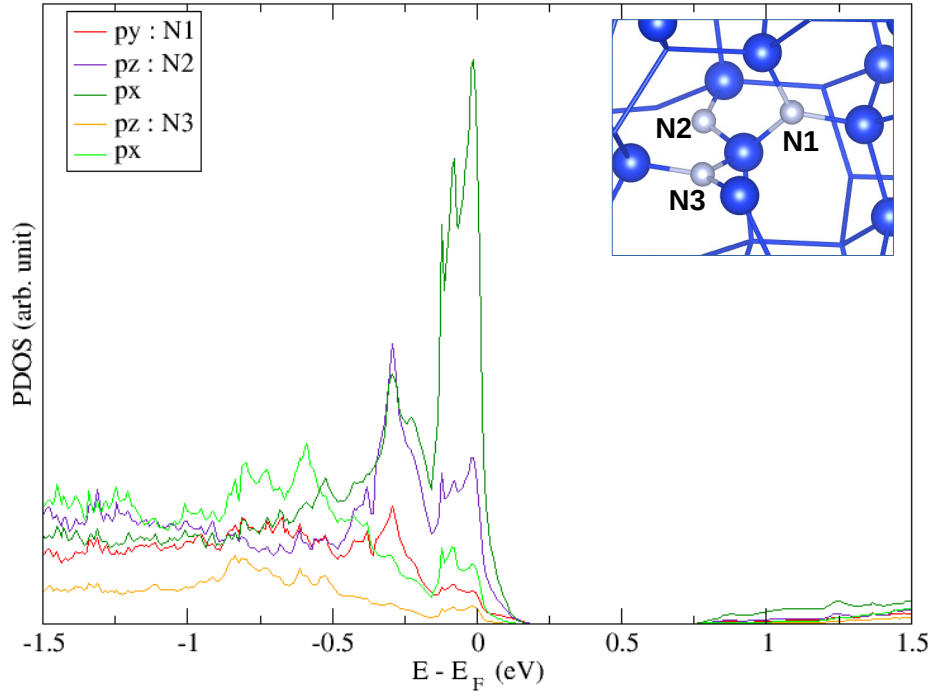

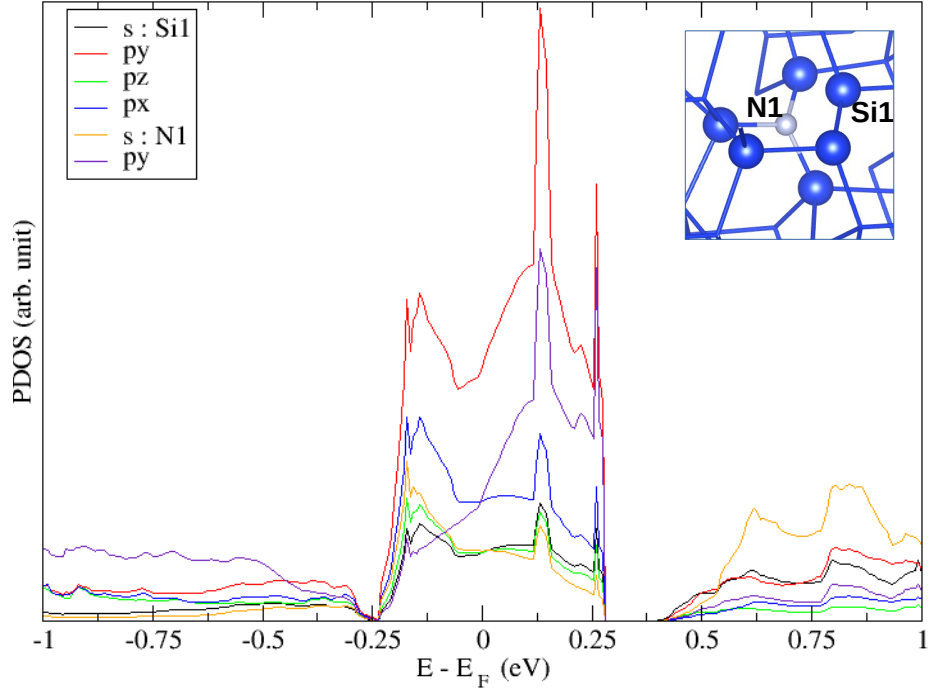

FIG. 11. Projected density of states (PDOS) of the atoms indicated in the inset structure, belonging to the  $\Sigma 3\{111\}$  with one interstitial N atom in presence of vacancy V2. The atomic orbitals with larger contributions are plotted here.

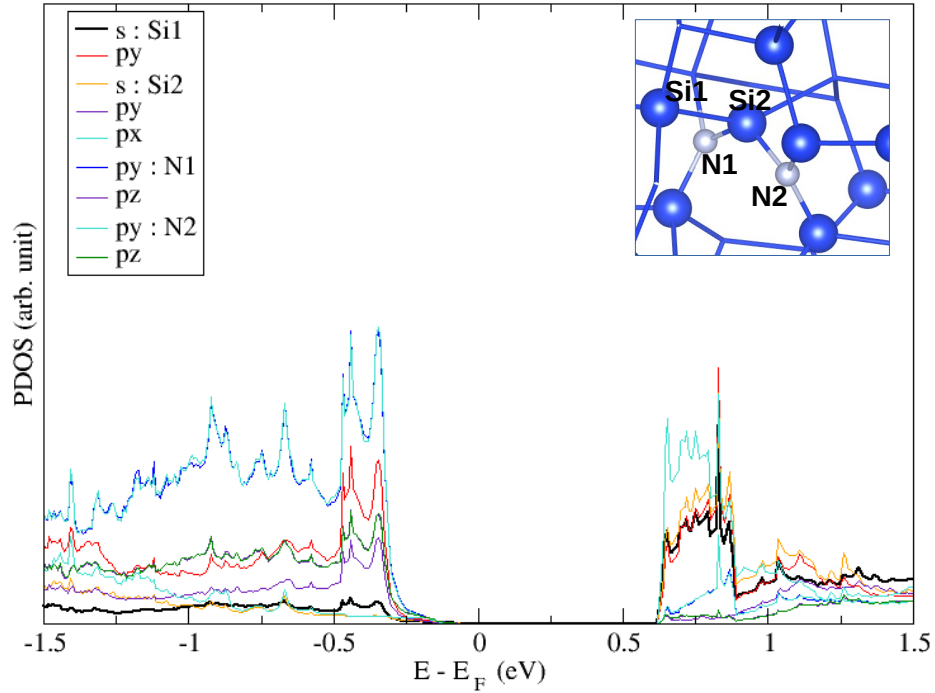

FIG. 12. Projected density of states (PDOS) of the atoms indicated in the inset structure, belonging to the  $\Sigma 3\{111\}$  with two interstitial N atoms in presence of vacancy V2. The atomic orbitals with larger contributions are plotted here.

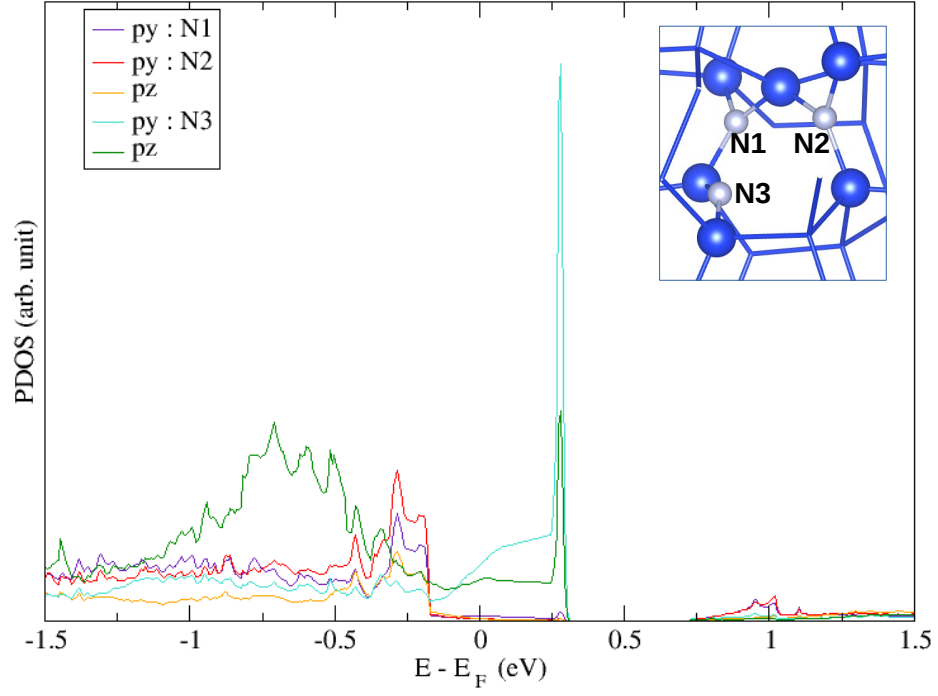

FIG. 13. Projected density of states (PDOS) of the atoms indicated in the inset structure, belonging to the  $\Sigma 3\{111\}$  with three interstitial N atoms in presence of vacancy V2. The atomic orbitals with larger contributions are plotted here.
